# Supplementary material for: On the dynamics of spicules and mass flows in the solar atmosphere
Source: arXiv:2110.10656 source file (2021-10-20)
Supplement: Supplementary file 1 [file appendixB.tex]

\chapter{Source Code}
\label{app:source}
\section{Implementation}
The \texttt{phduio} class is implemented in the following way:
\lstinputlisting[language = {[LaTeX]{TeX}}]{phduio.cls}
